# Supplementary material for: PIDLoc: Cross-View Pose Optimization Network Inspired by PID Controllers
Source: arXiv:2503.02388 source file (2025-03-04)
Supplement: Supplementary file 1 [file X_suppl.tex]

\clearpage
\setcounter{page}{1}
\maketitlesupplementary
\newcommand{\xmark}{\textsf{X}}

\setcounter{section}{0} 
\setcounter{table}{0} 
\setcounter{figure}{0}

\begin{comment}
    \section{Rationale}
\label{sec:rationale}
% 
Having the supplementary compiled together with the main paper means that:
% 
\begin{itemize}
\item The supplementary can back-reference sections of the main paper, for example, we can refer to \cref{sec:intro};
\item The main paper can forward reference sub-sections within the supplementary explicitly (e.g. referring to a particular experiment); 
\item When submitted to arXiv, the supplementary will already included at the end of the paper.
\end{itemize}
% 
To split the supplementary pages from the main paper, you can use \href{https://support.apple.com/en-ca/guide/preview/prvw11793/mac#:~:text=Delete%20a%20page%20from%20a,or%20choose%20Edit%20%3E%20Delete).}{Preview (on macOS)}, \href{https://www.adobe.com/acrobat/how-to/delete-pages-from-pdf.html#:~:text=Choose%20%E2%80%9CTools%E2%80%9D%20%3E%20%E2%80%9COrganize,or%20pages%20from%20the%20file.}{Adobe Acrobat} (on all OSs), as well as \href{https://superuser.com/questions/517986/is-it-possible-to-delete-some-pages-of-a-pdf-document}{command line tools}.
\end{comment}
\section{Implementation details}
%We provide additional implementation details in the experimental section~\ref{sec:experiments}. The resolutions of the ground-view images are $375\times 1242$ and $432\times816$ for the KITTI and FMAVS datasets, respectively. KITTI dataset은 one-to-one setting으로 실험하고 Ford Multi-AV Seasonal (FMAVS) dataset은 one-to-many으로 실험했다. 

We provide additional implementation details in Section~\ref{sec:experiments} (Experiments). The resolutions of the ground-view images are $375\times1242$ and $432\times816$ for the KITTI and FMAVS datasets, respectively. The experiments were conducted in the HighlyAccurate~\cite{shi2022beyond} and SIBCL~\cite{wang2023satellite} settings for the KITTI and FMAVS datasets, respectively.
Both the HighlyAccurate and SIBCL settings generate initial poses by adding noise to the ground-truth pose. In the HighlyAccurate setting, the initial pose is aligned to the satellite image center. In contrast, the SIBCL setting aligns the ground-truth pose to the satellite image center, which risks overfitting the model by biasing predictions toward the center. To ensure a fair comparison on the FMAVS dataset, we modified the SIBCL setting by not aligning the ground-truth pose to the center and reproduced previous works.

In the I branch, the search radius and step size of pose candidates are set to one-fourth of the noise range of the initial pose. This configuration generates two samples along the lateral, longitudinal, and azimuth directions; resulting in a total of six pose candidates. For example, if the noise range of the initial pose is $\pm 20\text{m}$, $\pm 20\text{m}$, and $\pm 10^\circ$, the search radius and step size are set to $10\text{m}$, $10\text{m}$, and $5^\circ$, respectively. Excluding the \tcolor{given} pose, two samples are generated in each direction: $+10\text{m}$ and $-10\text{m}$ in the position direction, and $+5^\circ$ and $-5^\circ$ in the orientation direction. To prevent gradient explosion during training, the gradients of the network parameters are clipped to a maximum $\ell_2\text{-norm}$ of $10$.
%For example, initial pose noise range가 $\pm{20}\text{m}$ and $\pm{10^\circ}$이라면 search radius와 step size는 $10\text{m}$ and $\pm{5^\circ}$이다. 현재 pose를 제외하고, position 방향으로는 $10\text{m}$ and $-10\text{m}$, orientation 방향으로는 $5^\circ$와 $-5^\circ$으로 각 방향에서 two samples을 활용하여 총 six samples를 pose candidate로 활용한다. Network parameter의 gradient는 10으로 clipping해서 gradient explosion을 방지한다. 

\section{Additional experiments}
\subsection{Ablation studies}
\paragraph{Impact of the coefficients of the PID branches}
%We evaluated the impact of the coefficients of the PID branches on the localization performance using the cross-view KITTI dataset. In conventional control theory, PID controllers are highly sensitive to the coefficients해서 gain tuning이라는 과정을 통해서 coefficient를 manually하게 찾는다. 하지만 제안한 방법은 coefficient를 learnable parameter로 설정해서 gain tuning과 같은 hyperparameter tuning을 필요로 하지 않는다. In Table~\ref{fig:subfig_a}, constant coefficients는 1로 설정했고, learnable coefficients는 1로 initialization해서 성능을 비교했다. learnable coefficients는 pid 계수가 1에서 각각 0.868, 0.930, 1.214로 학습 기반으로 tuning되어서, constant 경우와 비교해서 longitudinal 방향으로 $X\%\text{p}$의 성능 향상이 있다. 이는 각 branch 별로 중요도를 학습 기반으로 학습했기 때문이다. 
We evaluated the impact of the coefficients $k_p$, $k_i$, and $k_d$ of the PID branches on the localization performance using the cross-view KITTI dataset. In the conventional control theory, PID controllers are highly sensitive to the coefficients, requiring manual gain tuning to optimize the performance. In contrast, the proposed PIDLoc optimizes these coefficients through a learning-based approach, eliminating the need for manual hyperparameter tuning. 

Table~\ref{tab:pid_k_learnable} compares the performance of constant and learnable coefficients in the PID branches. The constant coefficients ($k_p$, $k_i$, $k_d$) are set to one and the learnable coefficients ($k_p$, $k_i$, $k_d$) are initialized to one. After the training, the learnable coefficients were tuned to $0.868$, $0.930$, and $1.214$, respectively. This learning-based tuning resulted in a lateral and longitudinal localization improvement of $1.50\%\text{p}$ and $1.08\%\text{p}$ compared with the constant coefficient baseline. The learnable coefficients adaptively capture the importance of each branch, improving the overall localization performance. 

Table~\ref{tab:pid_k} compares the impact of the coefficients on localization performance by fixing their values to some constants. The PID branches consistently improve position performance compared with the P, PI, and PD branches, demonstrating the effectiveness of including ID branches across various coefficient settings. Notably, configurations of ($k_p=0.5$, $k_i=1.0$, $k_d=1.0$) and ($k_p=1.0$, $k_i=1.0$, $k_d=1.5$) indicate that reducing $k_p$ improves lateral performance while increasing $k_d$ improves longitudinal performance. This result is consistent with the learnable coefficients of ($k_p=0.868$, $k_i=0.930$, $k_d=1.214$) in Table~\ref{tab:pid_k_learnable}, demonstrating that the learnable coefficients effectively capture the balance among the PID branches.

%추가적으로 Table~\ref{tab:pid_k}에서 각 branch에 대해서 coefficient의 영향을 확인할 수 있도록 coefficient를 0.5, 1, 1.5의 constant value로 설정해서 성능을 비교했다. PID branches는 다양한 PID 계수에서도 $k_d=0$ or $k_i=0$인 P, PI, and PD branches보다 성능이 모두 향상되었다. 또한, 다양한 PID 계수에서도 PID branches는 표준편차가 $X$로 안정적인 성능을 보여준다. Table~\ref{tab:pid_k_learnable}에서 learnable coefficients $k_p$, $k_i$, and $k_d$ were tuned to $0.868$, $0.930$, and $1.214$로 조정된 것과 같이, Table~\ref{tab:pid_k}에서도 $k_p$가 작고, $k_d$가 클 때 localization 성능이 향상된 것을 확인할 수 있다.
%ver2. 하지만 제안한 방법은 Table A에서 볼 수 있다시피, the coefficients of the PID branches에 sensitive하지 않기 때문에 gain tuning을 필요로 하지 않는다. Table A는 PID 계수를 각각 0.5, 1.5로 설정해서 학습한 결과를 보여준다. 다양한 PID branches의 계수에서 제안한 방법은 안정적인 성능을 보여주며, P branch 대비 모두 향상된 성능을 보여준다.

\begin{table}[t!]
    \begin{center}
    {\footnotesize 
        \setlength\tabcolsep{4pt}
        \begin{tabular}{@{} c *{8}{c}@{}}
            \toprule 
                \multicolumn{1}{c}{\multirow{2}{*}{Learnable}} & 
                \multicolumn{1}{c}{Lat. (\%) ↑} & 
                \multicolumn{1}{c}{Long. (\%) ↑} &
                \multicolumn{1}{c}{Orien. (\%) ↑}  
            \\ 
                \multicolumn{1}{c}{} &
                \multicolumn{1}{c}{R@$1\text{m}$} &
                \multicolumn{1}{c}{R@$1\text{m}$} &
                \multicolumn{1}{c}{R@$1^{\circ}$} \\ 
            \midrule
                \mc{\xmark} & 69.51 & 48.94 & 99.95\\ % c c c
                \mc{\checkmark} & \textbf{71.01} & \textbf{50.02} & \textbf{99.96} \\  % c * c 
            \bottomrule 
        \end{tabular}
    }
\caption{Comparison between constant and learnable coefficients in the PID branches.}
\label{tab:pid_k_learnable}
\end{center}
\end{table}
\begin{table}[t!]
\begin{center}
    {\footnotesize 
        \setlength\tabcolsep{4pt}
        \begin{tabular}{@{} c *{8}{c}@{}}
            \toprule 
                \multicolumn{1}{c}{\multirow{2}{*}{Branches}} &
                \multicolumn{1}{c}{\multirow{2}{*}{$k_p$}} &
                \multicolumn{1}{c}{\multirow{2}{*}{$k_i$}} &
                \multicolumn{1}{c}{\multirow{2}{*}{$k_d$}} &
                \multicolumn{1}{c}{Lat. (\%) ↑} & 
                \multicolumn{1}{c}{Long. (\%) ↑} &
                \multicolumn{1}{c}{Orien. (\%) ↑}  
            \\ 
                \multicolumn{1}{c}{} &
                \multicolumn{1}{c}{} &
                \multicolumn{1}{c}{} &
                \multicolumn{1}{c}{} &
                \multicolumn{1}{c}{R@$1\text{m}$} &
                \multicolumn{1}{c}{R@$1\text{m}$} &
                \multicolumn{1}{c}{R@$1^{\circ}$} \\ 
            \midrule
                \mc{P} & 1.0 & 0.0 & 0.0 & 66.67 & 41.03 & 99.93 \\ % 66.67 41.03 99.93
                \mc{PI} & 1.0 & 1.0 & 0.0 & 68.36 & 48.13 & 99.81 \\ % 68.36 49.13 99.81
                \mc{PD} & 1.0 & 0.0 & 1.0 & 67.92 & 46.78 & 99.96 \\ % 67.92 46.78 99.96
                \mc{PID} & 1.0 & 1.0 & 1.0 & 69.51 & 48.94 & 99.95 \\ % *69.51 *49.41 *99.95
                \mc{PID} & 0.5 & 1.0 & 1.0 & \textbf{69.94} & 49.82 & 99.88 \\ % 69.94 50.82 99.88 o
                \mc{PID} & 1.5 & 1.0 & 1.0 & 68.41 & 48.40 & 99.95 \\ % 68.24 47.40 99.95 
                \mc{PID} & 1.0 & 0.5 & 1.0 & 68.36 & 48.51 & 99.94 \\ % 67.36 47.51 99.94
                \mc{PID} & 1.0 & 1.5 & 1.0 & 68.45 & 49.41 & 99.95 \\ % *68.45 *49.41 *99.95
                \mc{PID} & 1.0 & 1.0 & 0.5 & 69.07 & 48.21 & \textbf{99.97} \\ % 69.07 44.38 99.97
                \mc{PID} & 1.0 & 1.0 & 1.5 & 68.40 & \textbf{49.93} & 99.89 \\ % 65.21 48.93 99.89
            \bottomrule 
        \end{tabular}
    }
\caption{Ablation analysis of the constant coefficients in the PID branches.}
\label{tab:pid_k}
\end{center}
\end{table}
\paragraph{Impact of pose candidates}
In Table~\ref{tab:pose_candidates}, we evaluated the impact of the number of pose candidates in the I branch under two initial pose error settings: $\pm 20\text{m}$ and $\pm 10^\circ$, and $\pm 30\text{m}$ and $\pm 15^\circ$. The number of pose candidates is set to zero, two, and four per direction. The case with zero candidate corresponds to the PD branches. 
%Note that in the main paper, experiments were conducted only with 2 pose candidates.
%ver2. Pose candidate의 최적 개수는 initial pose error에 따라 달랐다. $\pm 20\text{m}$에서는 각 direction 방향으로 2개, $\pm 30\text{m}$에서는 각 direction 방향으로 4개가 있을 때 가장 효과적이었다. Initial pose error가 크면 wider field of view (FoV)를 cover할 수 있도록 pose candidate가 많은 것이 좋다. 하지만 initial pose error가 $\pm20\text{m}$로 상대적으로 작은 경우 pose candidate가 너무 많으면 과도한 정보량으로 인한 trade-off로 성능이 하락하는 것을 알 수 있다.
%Initial pose error가 클 때, pose candiate가 많을수록 wider field of view (FoV)를 고려해서 성능이 향상된다. 반면, initial pose error가 $\pm20\text{m}$로 상대적으로 작은 경우에는 pose candidate가 너무 많으면 과도한 정보량으로 인한 trade-off로 성능이 하락하는 것을 알 수 있다.
%ver3. Table~\ref{tab:pose_candidates}에서 볼 수 있듯이, Pose candidate 개수가 증가할수록 모델의 성능은 더 증가하는 것을 보여준다. $\pm 20\text{m}$에서는 pose candidate가 0개인 경우와 비교해서 2개, 4개인 경우에 longitudinal 방향 성능이 각각 $X\%p$, $X\%p$ 성능이 향상되었다. 이는 더 많은 pose candidate를 활용할수록 모델이 global context를 더 잘 통합한다는 것을 보여준다.

Table~\ref{tab:pose_candidates} demonstrates that increasing the number of pose candidates significantly enhances localization performance. Specifically, under the $\pm 30\text{m}$ initial noise conditions, incorporating two and four pose candidates per direction improves longitudinal performance by $7.71\%\text{p}$ and $9.57\%\text{p}$, respectively, compared with the case of no pose candidates. The process of sampling pose candidates adds approximately $22\text{ms}$ of inference time and $0.15\text{GB}$ of GPU memory per candidate. 
%These results indicate that incorporating more pose candidates enables the model to integrate global context effectively, improving the localization performance.
These results indicate that incorporating more pose candidates enables the model to integrate global context effectively, but a balance is required to manage computational resources.

\begin{table}[t!]
\begin{center}
    {\footnotesize 
        \setlength\tabcolsep{4pt}
        \begin{tabular}{@{} c *{8}{c}@{}}
            \toprule 
                \multicolumn{1}{c}{Pose candidates} & 
                \multicolumn{1}{c}{\multirow{2}{*}{Pose noise}} & 
                \multicolumn{1}{c}{Lat. (\%) ↑} & 
                \multicolumn{1}{c}{Long. (\%) ↑} &
                \multicolumn{1}{c}{Orien. (\%) ↑}  
            \\ 
                \multicolumn{1}{c}{per direction} &
                \multicolumn{1}{c}{} &
                \multicolumn{1}{c}{R@$1\text{m}$} &
                \multicolumn{1}{c}{R@$1\text{m}$} &
                \multicolumn{1}{c}{R@$1^{\circ}$} \\ 
            \midrule
                \mc{0} & $\pm20\text{m}, \pm10^\circ$ & 67.90 & 46.80 & 99.91\\ % c c c
                \mc{2} & $\pm20\text{m}, \pm10^\circ$ & \textbf{71.01} & 50.02 & \textbf{99.96} \\  % c c c
                \mc{4} & $\pm20\text{m}, \pm10^\circ$ & 69.21 & \textbf{51.24} &  99.91 \\   % * * *
            \midrule
                \mc{0} & $\pm30\text{m}, \pm15^\circ$ & 60.60 & 29.37 & 97.46\\ % c c c
                \mc{2} & $\pm30\text{m}, \pm15^\circ$ & 62.12 & 37.08 & 97.54 \\  % c * c 
                \mc{4} & $\pm30\text{m}, \pm15^\circ$ & \textbf{62.24} & \textbf{38.94} & \textbf{98.46} \\   % * * *
            \bottomrule 
        \end{tabular}
    }
\caption{Ablation analysis of the number of the pose candidates in the I branch.}
\label{tab:pose_candidates}
\end{center}
\end{table}
\begin{table}[t!]
\begin{center}
    {\footnotesize 
        \setlength\tabcolsep{4pt}
        \begin{tabular}{@{} c *{8}{c}@{}}
            \toprule 
                \multicolumn{1}{c}{\multirow{2}{*}{Iterations}} & \multicolumn{1}{c}{Lat. (\%) ↑} & 
                \multicolumn{1}{c}{Long. (\%) ↑} &
                \multicolumn{1}{c}{Orien. (\%) ↑} & 
                \multicolumn{1}{c}{Inference time}  
            \\ 
                \multicolumn{1}{c}{} &
                \multicolumn{1}{c}{R@$1\text{m}$} &
                \multicolumn{1}{c}{R@$1\text{m}$} &
                \multicolumn{1}{c}{R@$1^{\circ}$} &
                \multicolumn{1}{c}{(ms)}  
                \\ 
            \midrule
                \mc{1} & 56.48 & 32.05 & 99.92 & 101 \\ 
                \mc{3} & 70.13 & 47.68 & 99.95 & 225\\  
                \mc{5} & 71.01 & 50.02 & \textbf{99.96} & 374 \\   
                \mc{7} & \textbf{72.45} & \textbf{51.24} & 99.62 & 473 \\   % * * *
            \bottomrule 
        \end{tabular}
    }
\caption{Impact of the iterations of the PIDLoc on the localization performance.}
\label{tab:iterations}
\end{center}
\end{table}
\paragraph{Impact of iterations}
In Table~\ref{tab:iterations}, we evaluated the impact of the iterations on localization performance using the cross-view KITTI dataset. The proposed PIDLoc iteratively refines the estimated pose toward the ground-truth pose by leveraging the cross-view features at the given pose. When increasing iterations from one to three, the recall rates were improved by $13.65\%\text{p}$ and $15.63\%\text{p}$ in the lateral and longitudinal directions, respectively. However, Table~\ref{tab:iterations} shows that performance gains diminish beyond five iterations, as the refinement process converges and additional iterations rarely provide new information for further pose adjustments. To balance the performance with computational efficiency, we adopt the five iterations as the default configuration.

\begin{figure*}[t!]
    \centering
    \includegraphics[width=\textwidth]{fig/figureA/figA_v0.3.pdf} 
    \caption{The PIDLoc performs localization by incorporating local, global, and fine-grained contexts. The green circular sector represents the ground truth pose. The blue arrow represents the position adjustment of the given pose during the single iteration. The length of the blue arrow indicates the position update size.
    Similar to existing methods, the P branch relies solely on the given pose, often resulting in the convergence to a local optimum. The I branch incorporates global context from diverse poses, enabling position updates toward the ground-truth pose across a wide range of initial poses. The D branch leverages gradients of feature differences to perform fine-grained pose adjustments.}
    \label{fig:supple_flow}
\end{figure*}
\begin{table}[t!]
\begin{center}
    {\footnotesize 
        \setlength\tabcolsep{4pt}
        \begin{tabular}{@{} c *{8}{c}@{}}
            \toprule 
                \multicolumn{1}{c}{\multirow{2}{*}{Branch}} & 
                \multicolumn{1}{c}{Parallel}  &
                \multicolumn{1}{c}{Inference time} & 
                \multicolumn{1}{c}{Memory} 
                \\
                \multicolumn{1}{c}{} &
                \multicolumn{1}{c}{candidates} &
                \multicolumn{1}{c}{(ms)} &
                \multicolumn{1}{c}{(GB)} 
                \\ 
            \midrule
                \mc{P branch} & - & 182 & 5.61\\ % c c c
                \mc{PD branches} & - & 251 & 6.41 \\  % c * c 
                \mc{PI branches} & \xmark & 370 & 6.53 \\
                \mc{PI branches} & \checkmark & 234 & 7.13 \\
                \mc{PID branches} & \xmark & 510 & 7.26 \\
                \mc{PID branches} & \checkmark & 374 & 7.32 \\
            \bottomrule 
        \end{tabular}
    }
\caption{Computational complexity analysis of the proposed PIDLoc.} \label{tab:computational_resources}
\end{center}
\end{table}
\subsection{Computational resources}
%PIDLoc의 각 branch에 따른 inference time per image와 gpu memory 소모량을 NVIDIA RTX A5000 1 GPU와 AMD EPYC 7453 28-Core Processor CPU에서 측정했다. P branch에 ID branches를 추가하면 inference time per image와 gpu memory가 모두 증가한다. iterative하게 pose candidate를 sampling을 수행하면 the inference time of the PIDLoc for each image is $510\text{ms}$, which is comparable to the $500\text{ms}$ of the HighlyAccurate~\cite{shi2022beyond}. GPU parallel processing으로 pose candidate를 sampling하면, the inference time of the PIDLoc for each image is $370\text{ms}$로, $1.23\%$ GPU memory 증가로 더 빠르게 추정할 수 있다. Iterative sampling과 parallel sampling 모두 동일한 방식으로 pose candidate를 선택하므로 recall rate와 error 성능의 변화는 없다.
We analyzed the computational complexity of the PIDLoc across different PID-branch configurations. The computational complexity was measured using inference time per image and GPU memory usage of the PIDLoc on an NVIDIA RTX A5000 GPU and an AMD EPYC 7453 28-Core Processor CPU. When performing iterative sampling of pose candidates, the inference time for the PID branches is $510\text{ms}$ per image, which is comparable to the $500\text{ms}$ reported for HighlyAccurate~\cite{shi2022beyond}. When performing GPU parallel processing for pose candidate sampling, the inference time for the PID branches is reduced to $374\text{ms}$ per image, achieving $26.67\%$ reduced inference time with only $0.83\%$ increase in GPU memory usage. Notably, both iterative and parallel sampling methods use the same approach for selecting pose candidates, ensuring consistent recall rates and localization performance. These results demonstrate the computational efficiency of the PIDLoc, enabling real-world applications such as autonomous navigation and robotics.

\section{Qualitative analysis}
\subsection{Pose update on the diverse initial poses}
\begin{comment}
    {
    \small
    \bibliographystyle{ieeenat_fullname}
    \bibliography{main}
}
\end{comment}
%P branch는 주어진 pose만 고려해서 a local optimum에 잘 빠지는 것을 확인할 수 있다. Ground-truth pose와 반대 방향으로 position을 잘못 예측하거나 update가 거의 되지 않는 local optimum에 빠진다. I branch는 다양한 pose에서의 넓은 FoV를 고려해서 ground-truth pose에서 멀리 떨어져도 global optimum에 수렴한다. P branch와 달리, ground-truth pose 방향으로 position을 update하고 local optimum에 거의 빠지지 않는다. 하지만 ground-truth pose에 가까운 영역에서는 정밀하게 pose를 추정하지 못한다. D branch는 feature difference gradients를 활용해서 정밀하게 position을 update한다. PI branches와 달리 주어진 pose에서의 feature difference gradients를 활용하므로 미세한 feature 변화를 감지해서 pose를 update한다.
Figure~\ref{fig:supple_flow} illustrates the position adjustment of the PID branches at a given pose. The P branch only focuses on the given pose, resulting in the convergence to a local optimum. Specifically, the P branch often predicts the position in the wrong direction or fails to update the pose when trapped in a local optimum. In contrast, the I branch incorporates the wider field of view (FoV) from the pose candidates, making them converge to the global optimum. The I branch successfully updates the position toward the ground-truth pose for most initial poses. However, it struggles to accurately update poses in regions near the ground-truth pose. The D branch utilizes feature difference gradients to update the position with high precision. The feature difference gradients capture subtle feature variations near the ground-truth pose, enabling accurate pose updates.

\begin{figure*}[ht!]
    \centering
    \includegraphics[width=\textwidth]{fig/figureB/figureB.pdf} 
    \caption{Visualization of localization results. The red, green, and blue circular sectors represent the current, ground-truth, and predicted pose, respectively. The blue line represents the iterative trajectory of predicted poses and the blud dot represents the predicted pose at each iteration. Compared with SIBCL~\cite{wang2023satellite}, PIDLoc more accurately finds the global optimum in a challenging environment with repetitive patterns.}
    \label{fig:supple_pose}
\end{figure*}
\subsection{Visualization of localization results}
%In Fig.~\ref{fig:qualitative}, we compared the SIBCL~\cite{wang2023satellite} with our PIDLoc under an initial pose error of $\pm{30}\text{m}$ and $\pm{15}^\circ$ on the KITTI dataset. Subfigures (a)-(d)는 lateral, longitudinal 방향으로 반복되는 pattern이 존재하는 예시이다. (a)와 같이 lateral 방향으로 initial pose error가 클 때, SIBCL은 local optimum에 수렴하지만 제안한 PIDLoc는 도로와 유사한 건물을 피해서 global optimum에 정확하게 수렴한다. (b)-(d) The SIBCL~\cite{wang2023satellite}는 lateral 방향은 정확하게 추정했지만 longitudinal 방향으로는 converges to a local optimum in repetitive patterns due to its limited FoV. In contrast, PIDLoc leverages global and fine-grained contexts, building facades and vegetation rows와 같이 구별하기 어려운 repetitive pattern에서도 정확하게 localization을 수행한다. 
In Figure~\ref{fig:supple_pose}, we compared the SIBCL~\cite{wang2023satellite} with our PIDLoc under an initial pose error of $\pm{30}\text{m}$ and $\pm{15}^\circ$ on the KITTI dataset. Figures~\ref{fig:supple_pose} (a)-(d) illustrate examples with repetitive patterns along the lateral and longitudinal directions. In case (a), where the initial lateral pose error is significant, the SIBCL only finds a local optimum. In contrast, the PIDLoc accurately finds the global optimum by avoiding buildings that resemble roads. Cases (b)-(d) show that the SIBCL accurately estimates the lateral direction but the estimation converges to a local optimum in the longitudinal direction. This limitation arises from its restricted FoV when dealing with repetitive patterns along the longitudinal direction. In contrast, the PIDLoc leverages global and fine-grained contexts, enabling accurate localization even in challenging scenarios with repetitive patterns, such as building facades and vegetation rows.

\begin{table}[t!]
    \begin{center}
    {\footnotesize 
        \setlength\tabcolsep{4pt}
        \begin{tabular}{@{} c *{8}{c}@{}}
            \toprule 
                \multicolumn{1}{c}{Positional} & 
                \multicolumn{1}{c}{Lat. (\%) ↑} & 
                \multicolumn{1}{c}{Long. (\%) ↑} &
                \multicolumn{1}{c}{Orien. (\%) ↑}  
            \\ 
                \multicolumn{1}{c}{Embedding} &
                \multicolumn{1}{c}{R@$1\text{m}$} &
                \multicolumn{1}{c}{R@$1\text{m}$} &
                \multicolumn{1}{c}{R@$1^{\circ}$} \\ 
            \midrule
                \mc{\xmark} & 66.06 & 42.37 & 99.88\\ % c c c
                \mc{\checkmark} & \textbf{71.01} & \textbf{50.02} & \textbf{99.96} \\  % c * c 
            \bottomrule 
        \end{tabular}
    }
\caption{Comparison of SPE with and without positional embedding.}
\label{tab:pid_k_learnable}
\end{center}
\end{table}
